# Supplementary material for: Learning with Exposure Constraints in Recommendation Systems
Source: arXiv:2302.01377 source file (2023-11-10)
Supplement: Supplementary file 1 [file theoremsTable.tex]

\section{Table of theorems}

\begin{table}[ht]
  \begin{center}
    \caption{Theorem's table}
    \label{tab:table}

    \begin{tabular}{c|c|c|c|l} % <-- Alignments: 1st column left, 2nd middle and 3rd right, with vertical lines in between
     Link & Theorem description & location & proof location in short appen. & proof location in long appen. \\ \hline
     Theorem~\ref{the_12321} & classical algs has $\Omega(T)$ regret & Section~\ref{sec:model} & Appendix~\ref{sec:appendin_secmodel} & in the short \\
     Theorem~\ref{theoremOAlg1} & $\OPT-\PIOPT\leq k\tau$ & Subsection~\ref{subsec:PIC algclass} & Appendix~\ref{sec:appendix_stochSec} & Appendix~\ref{Asubsec:pico appr opt} \\
     Theorem~\ref{thm:dp} & $\DP(Z)=\PIOPT(Z)$ & Subsection~\ref{subsec:dynProg} & Appendix~\ref{sec:appendix_stochSec} &  Appendix~\ref{Asubsec:thmdp} \\
     Lemma~\ref{MERruntime} & $\MER$ run time is $O(\tau^k)$ & Subsection~\ref{subsec:dynProg} &   &  Appendix~\ref{Asubsec:MERruntime} \\
     Prop~\ref{prop:badevent_ifonlyif} & line 5 in Alg~\ref{alg:lcbapprox234f} $\iff$ bad event & Subsection~\ref{subsec:lcb_approx} &  & Appendinx~\ref{Asubsec:bad event ifanfonlyif} \\
     Prop~\ref{prop:DOlalgiscommitted} & $\OR(Z)$ is committed to $Z$ & Subsection~\ref{Asubsec:DOAld commited} & {\rotem Appendix~\ref{sec:appendix_stochSec}(must)}  & in the short \\
     Theorem~\ref{thm:lcbz and pico z} & $\PIOPT(Z)\leq \OR(Z) + O(\nicefrac{nT}{\sqrt{\tau}})$ & Subsection~\ref{subsec:lcb_approx} & Appendix~\ref{sec:appendix_stochSec} & Appendix~\ref{Asubset:lcbz and pico z} \\
     Theorem~\ref{theoremMainRegret1} & $\mainAlg$ reward related to $\SSO$  & Subsection~\ref{subsec:EESalg} & Appendix~\ref{sec:appendix_learning} & Appendix~\ref{Asubsec:EES regret} \\
     Theorem~\ref{theMainLB} & regret lower bound $\Omega(T^{\nicefrac{2}{3}})$  & Subsection~\ref{subsec:lowerBound} & Appendix~\ref{sec:appendix_learning} & Appendix~\ref{Asubsec:lb regret} \\
     Theorem~\ref{theoremDelta} & unknown $\delta \rightarrow$ linear regret  & Subsection~\ref{subsec:unknown delta} &  & Appendix~\ref{Asubsec:thmdelta} \\
     Theorem~\ref{theMainLB2} & regret lower bound where $\tau>\Omega(T^{\nicefrac{2}{3}})$   & Subsection~\ref{subsec:longer phae length} &  & Appendix~\ref{Asubsec:lb regret} \\
      Theorem~\ref{theoremNPcompleteness}& planning its NP-Complete   & {\rotem Subsection~\ref{subsec:pick z}} & Appendix~\ref{subsec:shortappendix_matchNPC} & Appendix~\ref{Asubsec:np complete} \\
      & $\DOAlg(c(q),Z)$ run time= $O(\tau^3)$  & Subsection~\ref{subsec:lcb_approx} & Appendix~\ref{subsec:shortappendix_matchNPC} & Appendix~\ref{subsec:appendix_matching} \\
     Inequality~\eqref{eq:using match with slack approximates match} & $\DOAlg(\cv^+,Z) \geq \E_{\q}\left[ \DOAlg(c(\q),Z) \right] - O(n\sqrt{\tau})$ & Subsection~\ref{subsec:lcb_approx} &  & inside Appendix~\ref{Asubset:lcbz and pico z} \\
      & $\OPT-\PIOPT=\Omega(\tau)$ & Subsection~\ref{subsec:longer phae length} & & Appendix~\ref{subsubsec:lbpiopt}

    \end{tabular}

  \end{center}
\end{table}
